# Supplementary material for: Methods to Estimate Cryptic Sequence Complexity
Source: arXiv:2404.10854 source file (2024-05-31)
Supplement: Supplementary file 1 [file supplement.tex]

\section{Supplemental Material}

\section{Example} \label{sec:example}

example \citep{gropp1996high}
